# Supplementary material for: Conversion Layer Controls the Evolution of Magnetic Deflections Near the Alfven Surface
Source: arXiv:2601.22321 source file (2026-01-29)
Supplement: Supplementary file 1 [file AlfvenSurface_Supp.pdf]

Draft version January 29, 2026
Typeset using LaTeX default style in AASTeX62

# SUPPLEMENTAL MATERIAL

## 1. INTERVALS

The data used in this study is collected from many intervals from encounters 13-23. Although most are not shown separately in the main results, they were categorized separately as either sub-Alfvénic (Table 1), super-Alfvénic (Table 2), or near-Alfvénic (Table 3).

**Table 1.** Sub-Alfvénic intervals ($M_a < 1$)

| Encounter | Start Time (UTC) | End Time (UTC) |
|---|---|---|
| 13 | 2022-09-06 06:00 | 2022-09-06 16:00 |
| 13 | 2022-09-06 18:00 | 2022-09-07 12:00 |
| 14 | 2022-12-11 04:00 | 2022-12-11 16:00 |
| 15 | 2023-03-16 12:00 | 2023-03-17 06:00 |
| 16 | 2023-06-20 01:00 | 2023-06-21 01:00 |
| 17 | 2023-09-27 06:00 | 2023-09-27 15:00 |
| 18 | 2023-12-29 04:00 | 2023-12-29 14:00 |
| 19 | 2024-03-29 06:00 | 2024-03-29 21:00 |
| 20 | 2024-06-30 03:00 | 2024-06-30 18:00 |
| 21 | 2024-09-28 11:00 | 2024-09-28 18:00 |
| 22 | 2024-12-24 00:00 | 2024-12-25 00:00 |
| 23 | 2025-03-22 06:00 | 2025-03-23 12:00 |

**Table 2.** Super-Alfvénic intervals ($M_a > 1$)

| Encounter | Start Time (UTC) | End Time (UTC) |
|---|---|---|
| 13 | 2022-09-07 18:00 | 2022-09-08 18:00 |
| 14 | 2022-12-10 01:00 | 2022-12-10 09:00 |
| 15 | 2023-03-16 00:00 | 2023-03-16 11:00 |
| 16 | 2023-06-24 00:00 | 2023-06-25 00:00 |
| 17 | 2023-09-28 20:00 | 2023-09-30 09:00 |
| 18 | 2023-12-25 14:00 | 2023-12-25 23:00 |
| 19 | 2024-04-01 10:00 | 2024-04-02 01:00 |
| 20 | 2024-07-01 20:00 | 2024-07-03 00:00 |
| 21 | 2024-10-03 00:00 | 2024-10-03 12:00 |
| 23 | 2025-03-21 00:00 | 2025-03-22 03:00 |

**Table 3.** Near-Alfvénic intervals ($M_a \sim 1$)

| Encounter | Start Time (UTC) | End Time (UTC) |
|---|---|---|
| 13 | 2022-09-05 11:00 | 2022-09-05 17:00 |
| 16 | 2023-06-23 00:00 | 2023-06-23 18:00 |
| 17 | 2023-09-28 09:00 | 2023-09-28 18:00 |
| 18 | 2023-12-28 00:00 | 2023-12-29 00:00 |
| 19 | 2024-03-28 22:00 | 2024-03-29 05:00 |
| 20 | 2024-06-29 00:00 | 2024-06-29 09:00 |
| 21 | 2024-10-01 15:00 | 2024-10-02 00:00 |

## 2. DATA COVERAGE

Taking the intervals in the previous section together, this study consists of over 400 hours of PSP data. In figure 1 are histograms showing how that data is distributed with $\log_{10}(M_a)$ and with radial distance from the sun. Most of the collected data falls within the range $|\log_{10}(M_a)| \lesssim 0.5$, with roughly comparable amounts in the sub- and super-Alfvénic regimes.

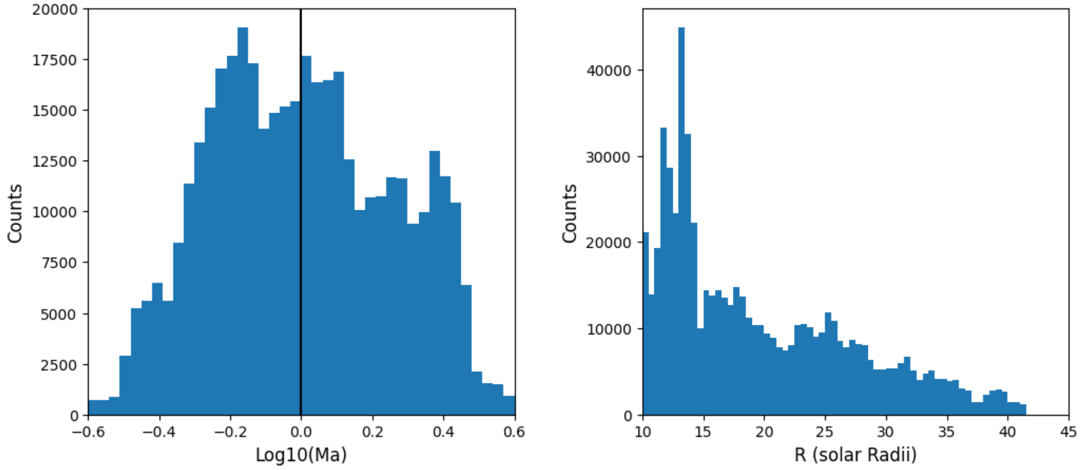


**Figure 1.** Data distribution with $\log_{10}(M_a)$ (left) and radial distance (right). The vertical black line in the left panel indicates the Alfvén surface which divides the sub- and super-Alfvénic regimes.
